# Supplementary material for: MERIT: Tensor Transform for Memory-Efficient Vision Processing on Parallel Architectures
Source: arXiv:1911.03458 source file (2019-11-07)
Supplement: Supplementary file 1 [file Appendix.pdf]

# I. About the formula to generate the address pattern

$$A_0 = 3,\ C_{0:2} = (1,2,12)$$

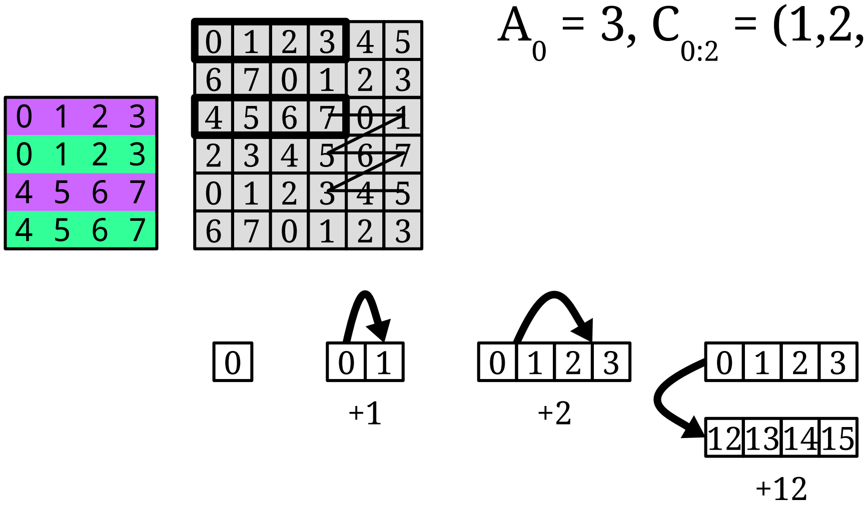

# II. Building hash property matrix **H**

$A_0 = 3, C_{0:2} = (1,6,12)$

| 3 | 4 | 1 | 2 | 7 | 0 | 5 | 6 | |
|---|---|---|---|---|---|---|---|---|
| 1 | 0 | 1 | 0 | 1 | 0 | 1 | 0 | Bit 0 |
| 1 | 0 | 0 | 1 | 1 | 0 | 0 | 1 | Bit 1 |
| 0 | 1 | 0 | 0 | 1 | 0 | 1 | 1 | Bit 2 |

| | | |
|---|---|---|
| 1 | 0 | 0 |
| X | 1 | 0 |
| X | X | 1 |

3+12 vs 3+12+1
The +1 always flips Bit 0, but the carry cannot be predicted , so the higher bits are X.

| 3 | 4 | 1 | 2 | 7 | 0 | 5 | 6 | |
|---|---|---|---|---|---|---|---|---|
| 1 | 0 | 1 | 0 | 1 | 0 | 1 | 0 | Bit 0 |
| 1 | 0 | 0 | 1 | 1 | 0 | 0 | 1 | Bit 1 |
| 0 | 1 | 0 | 0 | 1 | 0 | 1 | 1 | Bit 2 |

| | | |
|---|---|---|
| 1 | 0 | 0 |
| X | 1 | 0 |
| X | X | 1 |

3+6 vs 3+12
This pair is not constrainted according to the definition of **H**.

3+1+12 vs 3+1+6+12
Similarly, the +6 always flips Bit 1, but the higher bits are X.

# III. Uniqueness from matrix **H**

Prove by iteratively removing all possible conflicts.

$$A_0 = 3,\ C_{0:2} = (1,6,12)$$

| 3 | 4 | 1 | 2 | 7 | 0 | 5 | 6 | |
|---|---|---|---|---|---|---|---|---|
| 1 | 0 | 1 | 0 | 1 | 0 | 1 | 0 | Bit 0 |
| 1 | 0 | 0 | 1 | 1 | 0 | 0 | 1 | Bit 1 |
| 0 | 1 | 0 | 0 | 1 | 0 | 1 | 1 | Bit 2 |

| | | |
|---|---|---|
| 1 | 0 | 0 |
| X | 1 | 0 |
| X | X | 1 |

Remove an elementary row.

The 1 means we can remove 4 candidates since their Bit 0 is different from us.

| 3 | 4 | 1 | 2 | 7 | 0 | 5 | 6 | |
|---|---|---|---|---|---|---|---|---|
| 1 | 0 | 1 | 0 | 1 | 0 | 1 | 0 | Bit 0 |
| 1 | 0 | 0 | 1 | 1 | 0 | 0 | 1 | Bit 1 |
| 0 | 1 | 0 | 0 | 1 | 0 | 1 | 1 | Bit 2 |

| | | |
|---|---|---|
| 1 | 0 | 0 |
| X | 1 | 0 |
| X | X | 1 |

This time, the 1 means we can remove 2 candidates since their Bit 1 is different from us.

| 3 | 4 | 1 | 2 | 7 | 0 | 5 | 6 | |
|---|---|---|---|---|---|---|---|---|
| 1 | 0 | 1 | 0 | 1 | 0 | 1 | 0 | Bit 0 |
| 1 | 0 | 0 | 1 | 1 | 0 | 0 | 1 | Bit 1 |
| 0 | 1 | 0 | 0 | 1 | 0 | 1 | 1 | Bit 2 |

| | | |
|---|---|---|
| 1 | 0 | 0 |
| X | 1 | 0 |
| X | X | 1 |

Now we can remove the last candidate.

# IV. Butterfly network solvability from **H**

| 3 | 4 | 1 | 2 | 7 | 0 | 5 | 6 | |
|---|---|---|---|---|---|---|---|---|
| 1 | 0 | 1 | 0 | 1 | 0 | 1 | 0 | Bit 0 |
| 1 | 0 | 0 | 1 | 1 | 0 | 0 | 1 | Bit 1 |
| 0 | 1 | 0 | 0 | 1 | 0 | 1 | 1 | Bit 2 |

| | | |
|---|---|---|
| 1 | 0 | 0 |
| X | 1 | 0 |
| X | X | 1 |

Sub-problem 0 Sub-problem 0

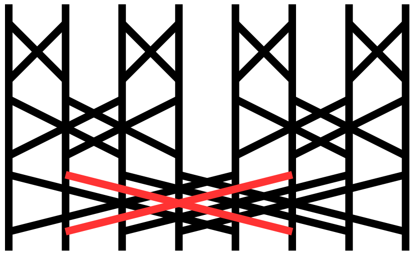

Sub-problem 0 Sub-problem 0

(Lower bits unchanged)

| 5 | 6 | 7 | 4 | 0 | 1 | 2 | 3 | |
|---|---|---|---|---|---|---|---|---|
| 1 | 0 | 1 | 0 | 0 | 1 | 0 | 1 | Bit 0 |
| 0 | 1 | 1 | 0 | 0 | 0 | 1 | 1 | Bit 1 |
| 1 | 1 | 1 | 1 | 0 | 0 | 0 | 0 | Bit 2 |

| | | |
|---|---|---|
| 1 | 0 | X |
| X | 1 | X |
| 0 | 0 | 1 |

Sub-problem 1 Sub-problem 2

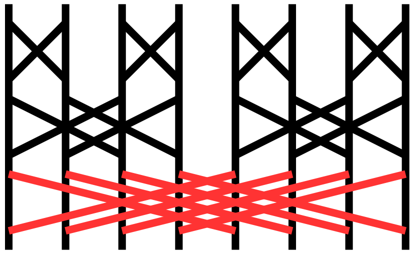

Sub-problem 2 Sub-problem 1

(Sub-problems are swapped)

## V. Circuit for **R** and **X**

| | | | | | | | | |
|---|---|---|---|---|---|---|---|---|
| 3 | 4 | 1 | 2 | 7 | 0 | 5 | 6 | |
| 1 | 0 | 1 | 0 | 1 | 0 | 1 | 0 | Bit 0 |
| 1 | 0 | 0 | 1 | 1 | 0 | 0 | 1 | Bit 1 |
| 0 | 1 | 0 | 0 | 1 | 0 | 1 | 1 | Bit 2 |

Sub-problem 0 Sub-problem 0

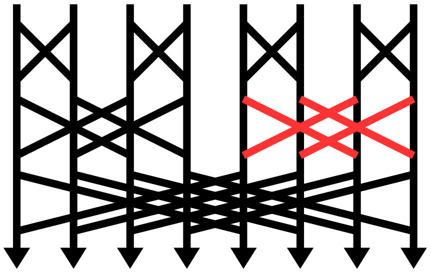

**X**

| | | | |
|---|---|---|---|
| 1 | 0 | 0 | 0 |
| 0 | 1 | 1 | 0 |
| 0 | 0 | 1 | 1 |

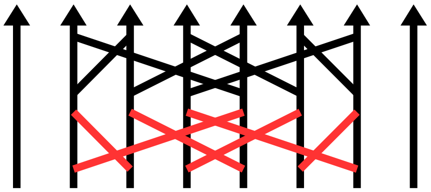

Swap 2 upper bits to bottom.

Swap 1 upper bits to bottom.

(Omega Network)

**R**[1]

| | | |
|---|---|---|
| 0 | 0 | 1 |
| 1 | 0 | 0 |
| 0 | 1 | 0 |
